# Supplementary material for: GaMO: Geometry-aware Multi-view Diffusion Outpainting for Sparse-View 3D Reconstruction
Source: arXiv:2512.25073 source file (2026-04-04)
Supplement: Supplementary file 1 [file suppl.tex]

\documentclass[runningheads]{llncs}
\PassOptionsToPackage{table}{xcolor} 
\usepackage[review,year=2026,ID=660]{eccv}

\usepackage{eccvabbrv}
\usepackage{makecell}
\usepackage{graphicx}
\usepackage{booktabs}
\usepackage{array}
\usepackage{enumitem}
\usepackage{subcaption}
\usepackage{gensymb}
\usepackage{arydshln}
\usepackage{multirow}
\usepackage{pifont}
\usepackage{xspace}
\usepackage{algorithm}
\usepackage{algorithmicx}
\usepackage{algpseudocode}
\usepackage{stfloats}
\usepackage{tabularx}
\usepackage{xstring}
\usepackage{url}
\usepackage[hang,flushmargin]{footmisc}
\usepackage{wrapfig}
\usepackage{placeins}
\usepackage[accsupp]{axessibility}
\usepackage{hyperref}
\usepackage{orcidlink}
\usepackage[table]{xcolor}
\usepackage{colortbl}

% TODO FINAL: Un-comment the following line for the camera-ready version
%\usepackage{eccv}

% OPTIONAL: Un-comment the following line for a version which is easier to read
% on small portrait-orientation screens (e.g., mobile phones, or beside other windows)
%\usepackage[mobile]{eccv}

\newlength\paramargin
\newlength\figmargin
\newlength\subfigmargin
\newlength\presecmargin
\newlength\secmargin
\newlength\subsecmargin
\newlength\subsubsecmargin
\newlength\tabmargin
\newlength\eqmargin
\newlength\paraskip

\setlength{\paramargin}{0mm}
\setlength{\figmargin}{-3mm}
\setlength{\subfigmargin}{0mm}
\setlength{\secmargin}{-.5em}
\setlength{\subsecmargin}{-.5em}
\setlength{\subsubsecmargin}{-.5em}
\setlength{\tabmargin}{-3mm}
\setlength{\eqmargin}{-1.5mm}

\setlength{\presecmargin}{0mm}
\setlength{\paraskip}{0mm}

% ---------------------------------------------------------------
% Other packages

\definecolor{ForestGreen}{RGB}{34,139,34}

\algrenewcommand\algorithmicrequire{\textbf{Input:}}
\algrenewcommand\algorithmicensure{\textbf{Output:}}

% ---------------------------------------------------------------
% Hyperref package

% It is strongly recommended to use hyperref, especially for the review version.
% Please disable hyperref *only* if you encounter grave issues.
% hyperref with option pagebackref eases the reviewers' job, but should be disabled for the final version.
%
% If you comment hyperref and then uncomment it, you should delete
% main.aux before re-running LaTeX.
% (Or just hit 'q' on the first LaTeX run, let it finish, and you
%  should be clear).

% TODO FINAL: Comment out the following line for the camera-ready version
%\usepackage[pagebackref,breaklinks,colorlinks,citecolor=eccvblue]{hyperref}
% TODO FINAL: Un-comment the following line for the camera-ready version

\begin{document}

% ---------------------------------------------------------------
% TODO REVIEW: Replace with your title
\title{Supplementary Material for GaMO} 

% TODO REVIEW: If the paper title is too long for the running head, you can set
% an abbreviated paper title here. If not, comment out.
\titlerunning{GaMO}

% TODO FINAL: Replace with your author list. 
% Include the authors' OCRID for the camera-ready version, if at all possible.
\author{First Author\inst{1}\orcidlink{0000-1111-2222-3333} \and
Second Author\inst{2,3}\orcidlink{1111-2222-3333-4444} \and
Third Author\inst{3}\orcidlink{2222--3333-4444-5555}}

% TODO FINAL: Replace with an abbreviated list of authors.
\authorrunning{F.~Author et al.}
% First names are abbreviated in the running head.
% If there are more than two authors, 'et al.' is used.

% TODO FINAL: Replace with your institution list.
\institute{Princeton University, Princeton NJ 08544, USA \and
Springer Heidelberg, Tiergartenstr.~17, 69121 Heidelberg, Germany
\email{lncs@springer.com}\\
\url{http://www.springer.com/gp/computer-science/lncs} \and
ABC Institute, Rupert-Karls-University Heidelberg, Heidelberg, Germany\\
\email{\{abc,lncs\}@uni-heidelberg.de}}

\maketitle

\input{11_appendix}

\clearpage
\bibliographystyle{splncs04}
\bibliography{main}
\end{document}
